# Supplementary material for: Far-Field Compression for Fast Kernel Summation Methods in High Dimensions
Source: arXiv:1409.2802 source file (2015-02-13)
Supplement: Supplementary file 1 [file appendix_experiments.tex]

%% Experiment stuff

\subsection{Quality of subsampling for kernel sub matrices}

Furthermore, the experiment has several sources of randomness -- the initial distribution of points, the choice of a center to form the source set $S$, and the randomness involved in the subsampling method.  Therefore, we should repeat any experiments many times and average over these trials. 

Several of these points require further thought and carefully justified choices.  In particular, many of them revolve around the interaction between the data, the choice of kernel, and our concept of far-field for the purposes of approximating interactions. 
\begin{itemize}
\item \textbf{Input Distribution} -- Currently, I have run many experiments on the multivariate Gaussian with unit covariance. This choice ties into the choice of kernel function and parameters.  Any other choices will require more thought about the kernel. One idea is to use real data here, along with some real kernels that make sense on the data (from the literature?)
\item \textbf{Well-separatedness} -- I'm just arbitrarily using parameters from the FMM here. I could also use standard ones from the FGT. However, a more justified choice will take some careful thought. 
\item \textbf{Kernel} -- This is the third leg of the problem.  The choice of kernel isn't that difficult, since I can just show experiments for a variety of commonly used kernels in KDE etc. However, the choice of bandwidth is extremely important.  I can currently exactly justify the use of Silverman's parameters for Gaussian data and a Gaussian kernel, but I'm more out in the open for other choices.  Possibilities: show results for a range of kernels that would be used in searching through cross-validation, actually do KDE and CV and find the optimal bandwidth choice from this, or take values used in the literature. 
\end{itemize}

\subsubsection{Gaussian Distribution and Kernel Experiments}

In these experiments, we fix a distribution (up to dimensionality), and the kernel and all of its parameters. The distribution $\mathcal{D}$ is taken to be the $d$-dimensional multivariate Gaussian with identity covariance. The kernel is the multivariate Gaussian kernel:
\begin{equation}
K_h(x, y) = \frac{1}{N h^d (2 \pi)^{\frac{d}{2}}} \exp \left( -\frac{1}{2 h^2} \|x - y\|^2 \right) 
\end{equation}
where the bandwidth $h$ is the asymptotically optimal bandwidth for this kernel and input distribution \cite{silverman}
\begin{equation}
h = \left[\frac{4 }{ (2 d + 1) N} \right]^{\frac{1}{d+4}}
\label{eqn_gaussian_bandwidth}
\end{equation}
where $N$ is the number of points drawn from $\mathcal{D}$.

We show results for experiments for varying values of $d$, $D_{WS}$ and $\epsilon$. The value of $N$ given in the figures represents the number of targets that satisfy the well-separatedness constraint given by $D_{WS}$. The labels on the points for importance sampling correspond to the rank of the approximation taken. All results are averaged over 15 independent trials. 
%\begin{table}[htbp]
%\caption{Results for Gaussian distribution and kernel with bandwidth given in Eqn.~\ref{eqn_gaussian_bandwidth}. $N = 10^6, D_{WS} = 2, m = 100$. \label{table_gaussian_dist_gaussian_kernel}}
%\begin{center}\footnotesize
%\renewcommand{\arraystretch}{1.3}
%\begin{tabular}{|c|c|c|c|c|c|c|}\hline
%$d$ & $N$ & $r$ & Sampling method  & Num trials & Avg.~Error (Eqn.~\ref{eqn_relative_approx_error}) & Std. Dev. Error \\ \hline
%1 & fill in &  & Importance ($N_s = ?$) & fill in & fill in  & fill in  \\ 
%2 & fill in & & Importance () & fill in & fill in & fill in  \\ \hline
%\end{tabular}
%\end{center}
%\end{table}

%%%%%%%%%%%%%%%%%%
% WS = 2

\begin{figure}[tbph]
        \centering
        \subfigure[$\epsilon = 10^{-2}$.]{\includegraphics[width=0.3\textwidth]{figures/comp_gaussian_labelled/dim_1_eps_-2_ws_2.eps}} 
        \subfigure[$\epsilon = 10^{-8}$.]{\includegraphics[width=0.3\textwidth]{figures/comp_gaussian_labelled/dim_1_eps_-8_ws_2.eps}} 
        \subfigure[$\epsilon = 10^{-14}$.]{\includegraphics[width=0.3\textwidth]{figures/comp_gaussian_labelled/dim_1_eps_-14_ws_2.eps}} 
\caption{Gaussian kernel compression experiments with $N = 10^6$, $m = 100$, $d = 1$, and $D_{WS} = 2$.
\label{fig_1d_gaussian_ws2}}
\end{figure}

\begin{figure}[tbph]
        \centering
        \subfigure[$\epsilon = 10^{-2}$.]{\includegraphics[width=0.3\textwidth]{figures/comp_gaussian_labelled/dim_2_eps_-2_ws_2.eps}} 
        \subfigure[$\epsilon = 10^{-8}$.]{\includegraphics[width=0.3\textwidth]{figures/comp_gaussian_labelled/dim_2_eps_-8_ws_2.eps}} 
        \subfigure[$\epsilon = 10^{-14}$.]{\includegraphics[width=0.3\textwidth]{figures/comp_gaussian_labelled/dim_2_eps_-14_ws_2.eps}} 
\caption{Gaussian kernel compression experiments with $N = 10^6$, $m = 100$, $d = 2$, and $D_{WS} = 2$.
\label{fig_2d_gaussian_ws2}}
\end{figure}

\begin{figure}[tbph]
        \centering
        \subfigure[$\epsilon = 10^{-2}$.]{\includegraphics[width=0.3\textwidth]{figures/comp_gaussian_labelled/dim_3_eps_-2_ws_2.eps}} 
        \subfigure[$\epsilon = 10^{-8}$.]{\includegraphics[width=0.3\textwidth]{figures/comp_gaussian_labelled/dim_3_eps_-8_ws_2.eps}} 
        \subfigure[$\epsilon = 10^{-14}$.]{\includegraphics[width=0.3\textwidth]{figures/comp_gaussian_labelled/dim_3_eps_-14_ws_2.eps}} 
\caption{Gaussian kernel compression experiments with $N = 10^6$, $m = 100$, $d = 3$, and $D_{WS} = 2$.
\label{fig_3d_gaussian_ws2}}
\end{figure}

\begin{figure}[tbph]
        \centering
        \subfigure[$\epsilon = 10^{-2}$.]{\includegraphics[width=0.3\textwidth]{figures/comp_gaussian_labelled/dim_4_eps_-2_ws_2.eps}} 
        \subfigure[$\epsilon = 10^{-8}$.]{\includegraphics[width=0.3\textwidth]{figures/comp_gaussian_labelled/dim_4_eps_-8_ws_2.eps}} 
        \subfigure[$\epsilon = 10^{-14}$.]{\includegraphics[width=0.3\textwidth]{figures/comp_gaussian_labelled/dim_4_eps_-14_ws_2.eps}} 
\caption{Gaussian kernel compression experiments with $N = 10^6$, $m = 100$, $d = 4$, and $D_{WS} = 2$.
\label{fig_4d_gaussian_ws2}}
\end{figure}

\begin{figure}[tbph]
        \centering
        \subfigure[$\epsilon = 10^{-2}$.]{\includegraphics[width=0.3\textwidth]{figures/comp_gaussian_labelled/dim_5_eps_-2_ws_2.eps}} 
        \subfigure[$\epsilon = 10^{-8}$.]{\includegraphics[width=0.3\textwidth]{figures/comp_gaussian_labelled/dim_5_eps_-8_ws_2.eps}} 
        \subfigure[$\epsilon = 10^{-14}$.]{\includegraphics[width=0.3\textwidth]{figures/comp_gaussian_labelled/dim_5_eps_-14_ws_2.eps}} 
\caption{Gaussian kernel compression experiments with $N = 10^6$, $m = 100$, $d = 5$, and $D_{WS} = 2$.
\label{fig_5d_gaussian_ws2}}
\end{figure}

%%%%%%%%%%%%%%%%%%%%%%%%%%%%%%%%%%%%%%%%

\begin{figure}[tbph]
        \centering
        \subfigure[$\epsilon = 10^{-2}$.]{\includegraphics[width=0.3\textwidth]{figures/comp_gaussian_labelled/dim_1_eps_-2_ws_3.eps}} 
        \subfigure[$\epsilon = 10^{-8}$.]{\includegraphics[width=0.3\textwidth]{figures/comp_gaussian_labelled/dim_1_eps_-8_ws_3.eps}} 
        \subfigure[$\epsilon = 10^{-14}$.]{\includegraphics[width=0.3\textwidth]{figures/comp_gaussian_labelled/dim_1_eps_-14_ws_3.eps}} 
\caption{Gaussian kernel compression experiments with $N = 10^6$, $m = 100$, $d = 1$, and $D_{WS} = 3$.
\label{fig_1d_gaussian_ws3}}
\end{figure}

\begin{figure}[tbph]
        \centering
        \subfigure[$\epsilon = 10^{-2}$.]{\includegraphics[width=0.3\textwidth]{figures/repeats_after_mc_error/id_gaussian_eps_-2_d_1.eps}} 
        \subfigure[$\epsilon = 10^{-8}$.]{\includegraphics[width=0.3\textwidth]{figures/repeats_after_mc_error/id_gaussian_eps_-8_d_1.eps}} 
        \subfigure[$\epsilon = 10^{-14}$.]{\includegraphics[width=0.3\textwidth]{figures/repeats_after_mc_error/id_gaussian_eps_-14_d_1.eps}} 
\caption{Gaussian kernel compression experiments with $N = 10^6$, $m = 100$, $d = 1$, and $D_{WS} = 3$. These are a repeat of the previous runs after adding the MC error estimate. Only included for comparison purposes.
\label{fig_1d_gaussian_ws3_redo}}
\end{figure}

\begin{figure}[tbph]
        \centering
        \subfigure[$\epsilon = 10^{-2}$.]{\includegraphics[width=0.3\textwidth]{figures/comp_gaussian_labelled/dim_2_eps_-2_ws_3.eps}} 
        \subfigure[$\epsilon = 10^{-8}$.]{\includegraphics[width=0.3\textwidth]{figures/comp_gaussian_labelled/dim_2_eps_-8_ws_3.eps}} 
        \subfigure[$\epsilon = 10^{-14}$.]{\includegraphics[width=0.3\textwidth]{figures/comp_gaussian_labelled/dim_2_eps_-14_ws_3.eps}} 
\caption{Gaussian kernel compression experiments with $N = 10^6$, $m = 100$, $d = 2$, and $D_{WS} = 3$.
\label{fig_2d_gaussian_ws3}}
\end{figure}

\begin{figure}[tbph]
        \centering
        \subfigure[$\epsilon = 10^{-2}$.]{\includegraphics[width=0.3\textwidth]{figures/repeats_after_mc_error/id_gaussian_eps_-2_d_2.eps}} 
        \subfigure[$\epsilon = 10^{-8}$.]{\includegraphics[width=0.3\textwidth]{figures/repeats_after_mc_error/id_gaussian_eps_-8_d_2.eps}} 
        \subfigure[$\epsilon = 10^{-14}$.]{\includegraphics[width=0.3\textwidth]{figures/repeats_after_mc_error/id_gaussian_eps_-14_d_2.eps}} 
\caption{Gaussian kernel compression experiments with $N = 10^6$, $m = 100$, $d = 2$, and $D_{WS} = 3$. These are a repeat of the previous runs after adding the MC error estimate. Only included for comparison purposes.
\label{fig_2d_gaussian_ws3_redo}}
\end{figure}

\begin{figure}[tbph]
        \centering
        \subfigure[$\epsilon = 10^{-2}$.]{\includegraphics[width=0.3\textwidth]{figures/comp_gaussian_labelled/dim_3_eps_-2_ws_3.eps}} 
        \subfigure[$\epsilon = 10^{-8}$.]{\includegraphics[width=0.3\textwidth]{figures/comp_gaussian_labelled/dim_3_eps_-8_ws_3.eps}} 
        \subfigure[$\epsilon = 10^{-14}$.]{\includegraphics[width=0.3\textwidth]{figures/comp_gaussian_labelled/dim_3_eps_-14_ws_3.eps}} 
\caption{Gaussian kernel compression experiments with $N = 10^6$, $m = 100$, $d = 3$, and $D_{WS} = 3$.
\label{fig_3d_gaussian_ws3}}
\end{figure}

\begin{figure}[tbph]
        \centering
        \subfigure[$\epsilon = 10^{-2}$.]{\includegraphics[width=0.3\textwidth]{figures/repeats_after_mc_error/id_gaussian_eps_-2_d_3.eps}} 
        \subfigure[$\epsilon = 10^{-8}$.]{\includegraphics[width=0.3\textwidth]{figures/repeats_after_mc_error/id_gaussian_eps_-8_d_3.eps}} 
        \subfigure[$\epsilon = 10^{-14}$.]{\includegraphics[width=0.3\textwidth]{figures/repeats_after_mc_error/id_gaussian_eps_-14_d_3.eps}} 
\caption{Gaussian kernel compression experiments with $N = 10^6$, $m = 100$, $d = 3$, and $D_{WS} = 3$. These are a repeat of the previous runs after adding the MC error estimate. Only included for comparison purposes.
\label{fig_3d_gaussian_ws3_redo}}
\end{figure}

\begin{figure}[tbph]
        \centering
        \subfigure[$\epsilon = 10^{-2}$.]{\includegraphics[width=0.3\textwidth]{figures/comp_gaussian_labelled/dim_4_eps_-2_ws_3.eps}} 
        \subfigure[$\epsilon = 10^{-8}$.]{\includegraphics[width=0.3\textwidth]{figures/comp_gaussian_labelled/dim_4_eps_-8_ws_3.eps}} 
        \subfigure[$\epsilon = 10^{-14}$.]{\includegraphics[width=0.3\textwidth]{figures/comp_gaussian_labelled/dim_4_eps_-14_ws_3.eps}} 
\caption{Gaussian kernel compression experiments with $N = 10^6$, $m = 100$, $d = 4$, and $D_{WS} = 3$.
\label{fig_4d_gaussian_ws3}}
\end{figure}

\begin{figure}[tbph]
        \centering
        \subfigure[$\epsilon = 10^{-2}$.]{\includegraphics[width=0.3\textwidth]{figures/repeats_after_mc_error/id_gaussian_eps_-2_d_4.eps}} 
        \subfigure[$\epsilon = 10^{-8}$.]{\includegraphics[width=0.3\textwidth]{figures/repeats_after_mc_error/id_gaussian_eps_-8_d_4.eps}} 
        \subfigure[$\epsilon = 10^{-14}$.]{\includegraphics[width=0.3\textwidth]{figures/repeats_after_mc_error/id_gaussian_eps_-14_d_4.eps}} 
\caption{Gaussian kernel compression experiments with $N = 10^6$, $m = 100$, $d = 4$, and $D_{WS} = 3$. These are a repeat of the previous runs after adding the MC error estimate. Only included for comparison purposes.
\label{fig_4d_gaussian_ws3_redo}}
\end{figure}

\begin{figure}[tbph]
        \centering
        \subfigure[$\epsilon = 10^{-2}$.]{\includegraphics[width=0.3\textwidth]{figures/comp_gaussian_labelled/dim_5_eps_-2_ws_3.eps}} 
        \subfigure[$\epsilon = 10^{-8}$.]{\includegraphics[width=0.3\textwidth]{figures/comp_gaussian_labelled/dim_5_eps_-8_ws_3.eps}} 
        \subfigure[$\epsilon = 10^{-14}$.]{\includegraphics[width=0.3\textwidth]{figures/comp_gaussian_labelled/dim_5_eps_-14_ws_3.eps}} 
\caption{Gaussian kernel compression experiments with $N = 10^6$, $m = 100$, $d = 5$, and $D_{WS} = 3$.
\label{fig_5d_gaussian_ws3}}
\end{figure}

\begin{figure}[tbph]
        \centering
        \subfigure[$\epsilon = 10^{-2}$.]{\includegraphics[width=0.3\textwidth]{figures/repeats_after_mc_error/id_gaussian_eps_-2_d_5.eps}} 
        \subfigure[$\epsilon = 10^{-8}$.]{\includegraphics[width=0.3\textwidth]{figures/repeats_after_mc_error/id_gaussian_eps_-8_d_5.eps}} 
        \subfigure[$\epsilon = 10^{-14}$.]{\includegraphics[width=0.3\textwidth]{figures/repeats_after_mc_error/id_gaussian_eps_-14_d_5.eps}} 
\caption{Gaussian kernel compression experiments with $N = 10^6$, $m = 100$, $d = 5$, and $D_{WS} = 3$. These are a repeat of the previous runs after adding the MC error estimate. Only included for comparison purposes.
\label{fig_5d_gaussian_ws3_redo}}
\end{figure}

%%%%%%%%%%%%%%%%%%%%%%%%%%%%%%%%%%%%
%%%%%%%%%%%%%%
%WS = 4

\begin{figure}[tbph]
        \centering
        \subfigure[$\epsilon = 10^{-2}$.]{\includegraphics[width=0.3\textwidth]{figures/comp_gaussian_labelled/dim_1_eps_-2_ws_4.eps}} 
        \subfigure[$\epsilon = 10^{-8}$.]{\includegraphics[width=0.3\textwidth]{figures/comp_gaussian_labelled/dim_1_eps_-8_ws_4.eps}} 
        \subfigure[$\epsilon = 10^{-14}$.]{\includegraphics[width=0.3\textwidth]{figures/comp_gaussian_labelled/dim_1_eps_-14_ws_4.eps}} 
\caption{Gaussian kernel compression experiments with $N = 10^6$, $m = 100$, $d = 1$, and $D_{WS} = 4$.
\label{fig_1d_gaussian_ws4}}
\end{figure}

\begin{figure}[tbph]
        \centering
        \subfigure[$\epsilon = 10^{-2}$.]{\includegraphics[width=0.3\textwidth]{figures/comp_gaussian_labelled/dim_2_eps_-2_ws_4.eps}} 
        \subfigure[$\epsilon = 10^{-8}$.]{\includegraphics[width=0.3\textwidth]{figures/comp_gaussian_labelled/dim_2_eps_-8_ws_4.eps}} 
        \subfigure[$\epsilon = 10^{-14}$.]{\includegraphics[width=0.3\textwidth]{figures/comp_gaussian_labelled/dim_2_eps_-14_ws_4.eps}} 
\caption{Gaussian kernel compression experiments with $N = 10^6$, $m = 100$, $d = 2$, and $D_{WS} = 4$.
\label{fig_2d_gaussian_ws4}}
\end{figure}

\begin{figure}[tbph]
        \centering
        \subfigure[$\epsilon = 10^{-2}$.]{\includegraphics[width=0.3\textwidth]{figures/comp_gaussian_labelled/dim_3_eps_-2_ws_4.eps}} 
        \subfigure[$\epsilon = 10^{-8}$.]{\includegraphics[width=0.3\textwidth]{figures/comp_gaussian_labelled/dim_3_eps_-8_ws_4.eps}} 
        \subfigure[$\epsilon = 10^{-14}$.]{\includegraphics[width=0.3\textwidth]{figures/comp_gaussian_labelled/dim_3_eps_-14_ws_4.eps}} 
\caption{Gaussian kernel compression experiments with $N = 10^6$, $m = 100$, $d = 3$, and $D_{WS} = 4$.
\label{fig_3d_gaussian_ws4}}
\end{figure}

\begin{figure}[tbph]
        \centering
        \subfigure[$\epsilon = 10^{-2}$.]{\includegraphics[width=0.3\textwidth]{figures/comp_gaussian_labelled/dim_4_eps_-2_ws_4.eps}} 
        \subfigure[$\epsilon = 10^{-8}$.]{\includegraphics[width=0.3\textwidth]{figures/comp_gaussian_labelled/dim_4_eps_-8_ws_4.eps}} 
        \subfigure[$\epsilon = 10^{-14}$.]{\includegraphics[width=0.3\textwidth]{figures/comp_gaussian_labelled/dim_4_eps_-14_ws_4.eps}} 
\caption{Gaussian kernel compression experiments with $N = 10^6$, $m = 100$, $d = 4$, and $D_{WS} = 4$.
\label{fig_4d_gaussian_ws4}}
\end{figure}

\begin{figure}[tbph]
        \centering
        \subfigure[$\epsilon = 10^{-2}$.]{\includegraphics[width=0.3\textwidth]{figures/comp_gaussian_labelled/dim_5_eps_-2_ws_4.eps}} 
        \subfigure[$\epsilon = 10^{-8}$.]{\includegraphics[width=0.3\textwidth]{figures/comp_gaussian_labelled/dim_5_eps_-8_ws_4.eps}} 
        \subfigure[$\epsilon = 10^{-14}$.]{\includegraphics[width=0.3\textwidth]{figures/comp_gaussian_labelled/dim_5_eps_-14_ws_4.eps}} 
\caption{Gaussian kernel compression experiments with $N = 10^6$, $m = 100$, $d = 5$, and $D_{WS} = 4$.
\label{fig_5d_gaussian_ws4}}
\end{figure}

%%%%%

\clearpage

\begin{figure}[tbph]
        \centering
        \subfigure[$\epsilon = 10^{-2}$.]{\includegraphics[width=0.3\textwidth]{figures/comp_gaussian_labelled/dim_8_eps_-2_ws_3.eps}} 
        \subfigure[$\epsilon = 10^{-8}$.]{\includegraphics[width=0.3\textwidth]{figures/comp_gaussian_labelled/dim_8_eps_-8_ws_3.eps}} 
        \subfigure[$\epsilon = 10^{-14}$.]{\includegraphics[width=0.3\textwidth]{figures/comp_gaussian_labelled/dim_8_eps_-14_ws_3.eps}} 
\caption{Gaussian kernel compression experiments with $N = 10^6$, $m = 100$, $d = 8$, and $D_{WS} = 3$.
\label{fig_8d_gaussian_ws3}}
\end{figure}

\begin{figure}[tbph]
        \centering
        \subfigure[$\epsilon = 10^{-2}$.]{\includegraphics[width=0.3\textwidth]{figures/repeats_after_mc_error/id_gaussian_eps_-2_d_8.eps}} 
        \subfigure[$\epsilon = 10^{-8}$.]{\includegraphics[width=0.3\textwidth]{figures/repeats_after_mc_error/id_gaussian_eps_-8_d_8.eps}} 
        \subfigure[$\epsilon = 10^{-14}$.]{\includegraphics[width=0.3\textwidth]{figures/repeats_after_mc_error/id_gaussian_eps_-14_d_8.eps}} 
\caption{Gaussian kernel compression experiments with $N = 10^6$, $m = 100$, $d = 8$, and $D_{WS} = 3$. These are a repeat of the previous runs after adding the MC error estimate. Only included for comparison purposes.
\label{fig_8d_gaussian_ws3_redo}}
\end{figure}

\begin{figure}[tbph]
        \centering
        \subfigure[$\epsilon = 10^{-2}$.]{\includegraphics[width=0.3\textwidth]{figures/comp_gaussian_labelled/dim_10_eps_-2_ws_3.eps}} 
        \subfigure[$\epsilon = 10^{-8}$.]{\includegraphics[width=0.3\textwidth]{figures/comp_gaussian_labelled/dim_10_eps_-8_ws_3.eps}} 
        \subfigure[$\epsilon = 10^{-14}$.]{\includegraphics[width=0.3\textwidth]{figures/comp_gaussian_labelled/dim_10_eps_-14_ws_3.eps}} 
\caption{Gaussian kernel compression experiments with $N = 10^6$, $m = 100$, $d = 10$, and $D_{WS} = 3$.
\label{fig_10d_gaussian_ws3}}
\end{figure}

\begin{figure}[tbph]
        \centering
        \subfigure[$\epsilon = 10^{-2}$.]{\includegraphics[width=0.3\textwidth]{figures/repeats_after_mc_error/id_gaussian_eps_-2_d_10.eps}} 
        \subfigure[$\epsilon = 10^{-8}$.]{\includegraphics[width=0.3\textwidth]{figures/repeats_after_mc_error/id_gaussian_eps_-8_d_10.eps}} 
        \subfigure[$\epsilon = 10^{-14}$.]{\includegraphics[width=0.3\textwidth]{figures/repeats_after_mc_error/id_gaussian_eps_-14_d_10.eps}} 
\caption{Gaussian kernel compression experiments with $N = 10^6$, $m = 100$, $d = 10$, and $D_{WS} = 3$. These are a repeat of the previous runs after adding the MC error estimate. Only included for comparison purposes.
\label{fig_10d_gaussian_ws3_redo}}
\end{figure}

\begin{figure}[tbph]
        \centering
        \subfigure[$\epsilon = 10^{-2}$.]{\includegraphics[width=0.3\textwidth]{figures/repeats_after_mc_error/id_gaussian_eps_-2_d_15.eps}} 
        \subfigure[$\epsilon = 10^{-8}$.]{\includegraphics[width=0.3\textwidth]{figures/repeats_after_mc_error/id_gaussian_eps_-8_d_15.eps}} 
        \subfigure[$\epsilon = 10^{-14}$.]{\includegraphics[width=0.3\textwidth]{figures/repeats_after_mc_error/id_gaussian_eps_-14_d_15.eps}} 
\caption{Gaussian kernel compression experiments with $N = 10^6$, $m = 100$, $d = 15$, and $D_{WS} = 3$. These are a repeat of the previous runs after adding the MC error estimate. 
\label{fig_15d_gaussian_ws3_redo}}
\end{figure}

\subsection{Comparison against SVD}

We choose $N$ points from a  $d$ dimensional Gaussian distribution with covariance equal to the identity as before. We use a Gaussian kernel with asymptotically optimal bandwidth. We divide the points into sources and targets as before, compute the matrix $K$ of interactions between sources and targets, and subsample the rows of this matrix to form $K_s$. We then compress the matrix with the SVD.  

More concretely, given a tolerance $\epsilon$, we find the smallest rank $k$ such that $\sigma_{k+1} (K_s) < \epsilon \cdot \sigma_1 (K_s)$.  We then compute the first $k$ right singular vectors of $K_s$, $V_k$.  We compute the error as 
\begin{equation}
\frac{\|K - K V_k V_k^T\|}{\|K\|}
\label{eqn_svd_truncation_error}
\end{equation}

We plot these errors for all three sampling methods for a range of values of $\epsilon$ and $s$ as before. Note that these experiments are not currently averaged over multiple runs due to time constraints.

\begin{figure}[tbph]
        \centering
        \subfigure[$\epsilon = 10^{-2}$.]{\includegraphics[width=0.3\textwidth]{figures/svd_gaussian/dim_3_eps_-2_ws_2.eps}} 
        \subfigure[$\epsilon = 10^{-8}$.]{\includegraphics[width=0.3\textwidth]{figures/svd_gaussian/dim_3_eps_-8_ws_2.eps}} 
        \subfigure[$\epsilon = 10^{-14}$.]{\includegraphics[width=0.3\textwidth]{figures/svd_gaussian/dim_3_eps_-14_ws_2.eps}} 
\caption{Gaussian kernel SVD compression experiments with $N = 10^6$, $m = 100$, $d = 3$, and $D_{WS} = 2$.
\label{fig_3d_gaussian_ws2_svd}}
\end{figure}

\begin{figure}[tbph]
        \centering
        \subfigure[$\epsilon = 10^{-2}$.]{\includegraphics[width=0.3\textwidth]{figures/svd_gaussian/dim_3_eps_-2_ws_3.eps}} 
        \subfigure[$\epsilon = 10^{-8}$.]{\includegraphics[width=0.3\textwidth]{figures/svd_gaussian/dim_3_eps_-8_ws_3.eps}} 
        \subfigure[$\epsilon = 10^{-14}$.]{\includegraphics[width=0.3\textwidth]{figures/svd_gaussian/dim_3_eps_-14_ws_3.eps}} 
\caption{Gaussian kernel SVD compression experiments with $N = 10^6$, $m = 100$, $d = 3$, and $D_{WS} = 3$.
\label{fig_3d_gaussian_ws3_svd}}
\end{figure}

We also perform these experiments for the Laplace ($1/r$) kernel. 

\begin{figure}[tbph]
        \centering
        \subfigure[$\epsilon = 10^{-2}$.]{\includegraphics[width=0.3\textwidth]{figures/svd_laplace/svd_dim_3_eps_-2_ws_4.eps}} 
        \subfigure[$\epsilon = 10^{-8}$.]{\includegraphics[width=0.3\textwidth]{figures/svd_laplace/svd_dim_3_eps_-8_ws_4.eps}} 
        \subfigure[$\epsilon = 10^{-14}$.]{\includegraphics[width=0.3\textwidth]{figures/svd_laplace/svd_dim_3_eps_-14_ws_4.eps}} 
\caption{Laplace kernel SVD compression experiments with $N = 10^6$, $m = 100$, $d = 3$, and $D_{WS} = 4$.
\label{fig_3d_laplace_ws4_svd}}
\end{figure}

%%%%%%%%%%%%%%%%%%%%%%%%%%%%%%%%%%%%%%%%%%%%%%%%%%%%%
%%%%%%%%%%%%%%%%%%%%%%%%%%%%%%%%%%%%%%%%%%%%%%%%%%%%%
%%%%%%%%%%%%%%%%%%%%%%%%%%%%%%%%%%%%%%%%%%%%%%%%%%%%%
%%%%%%%%%%%%%%%%%%%%%%%%%%%%%%%%%%%%%%%%%%%%%%%%%%%%%

\subsection{Comparisons Against MC Subsampled Error}

We would like to examine experiments for which the number of sources $m$ increases.  However, the computational cost makes this prohibitive. Therefore, we resort to estimating the true error.  We have some true kernel matrix $K$ and compute an approximation $\hat{K}$ through any of the methods described previously.  We then choose an MC error sampling parameter $s$, and sample rows of $K$ from a Bernoulli distribution with parameter $s$.  Let this matrix be $K_s$.  Then, we report the estimated error:
\begin{equation}
\epsilon_{\textrm{MC}} = \frac{\|K_s - \hat{K}_s\|_2}{\|K_s\|_2}
\end{equation}
We can repeat these experiments $n_{\textrm{MC}}$ times. 

These experiments are also using reconfigured sampling methods.  
\begin{itemize}
\item \textbf{Bernoulli} -- A weighted coin is tossed for each row. The row is kept if the outcome is heads. 
\item \textbf{Uniform with replacement} -- For sampling parameter $s$, we take a sample of $\lceil s \cdot N \rceil$ rows uniformly with replacement.
\item \textbf{Uniform without replacement} -- For sampling parameter $s$, we take a sample of $\lceil s \cdot N \rceil$ rows uniformly with replacement.
\item \textbf{Euclidean with replacement} -- For sampling parameter $s$, we take a sample of $\lceil s \cdot N \rceil$ rows with probability proportional to their Euclidean lengths with replacement. 
\item \textbf{Euclidean without replacement} -- For sampling parameter $s$, we take a sample of $\lceil s \cdot N \rceil$ rows with probability proportional to their Euclidean lengths without replacement. 
\end{itemize}

Our first experiments use the parameter $s = 10^{-2}$ and $n_{\textrm{MC}} = 1$ for convenience. 

\begin{figure}[tbph]
        \centering
        \subfigure[$\epsilon = 10^{-2}$.]{\includegraphics[width=0.3\textwidth]{figures/mc_error_verification/id_gaussian_eps_-2.eps}} 
        \subfigure[$\epsilon = 10^{-8}$.]{\includegraphics[width=0.3\textwidth]{figures/mc_error_verification/id_gaussian_eps_-8.eps}} 
        \subfigure[$\epsilon = 10^{-14}$.]{\includegraphics[width=0.3\textwidth]{figures/mc_error_verification/id_gaussian_eps_-14.eps}} 
\caption{Gaussian kernel ID compression experiments with $N = 10^6$, $m = 100$, $d = 3$, and $D_{WS} = 4$. The error is computed exactly.
\label{fig_3d_gaussian_ws4_id_exact_error}}
\end{figure}

\begin{figure}[tbph]
        \centering
        \subfigure[$\epsilon = 10^{-2}$.]{\includegraphics[width=0.3\textwidth]{figures/mc_error_verification/svd_gaussian_eps_-2.eps}} 
        \subfigure[$\epsilon = 10^{-8}$.]{\includegraphics[width=0.3\textwidth]{figures/mc_error_verification/svd_gaussian_eps_-8.eps}} 
        \subfigure[$\epsilon = 10^{-14}$.]{\includegraphics[width=0.3\textwidth]{figures/mc_error_verification/svd_gaussian_eps_-14.eps}} 
\caption{Gaussian kernel SVD compression experiments with $N = 10^6$, $m = 100$, $d = 3$, and $D_{WS} = 4$. The error is computed exactly.
\label{fig_3d_gaussian_ws4_svd_exact_error}}
\end{figure}

\begin{figure}[tbph]
        \centering
        \subfigure[$\epsilon = 10^{-2}$.]{\includegraphics[width=0.3\textwidth]{figures/mc_error_verification/id_laplace_eps_-2.eps}} 
        \subfigure[$\epsilon = 10^{-8}$.]{\includegraphics[width=0.3\textwidth]{figures/mc_error_verification/id_laplace_eps_-8.eps}} 
        \subfigure[$\epsilon = 10^{-14}$.]{\includegraphics[width=0.3\textwidth]{figures/mc_error_verification/id_laplace_eps_-14.eps}} 
\caption{Laplace kernel ID compression experiments with $N = 10^6$, $m = 100$, $d = 3$, and $D_{WS} = 4$. The error is computed exactly.
\label{fig_3d_laplace_ws4_id_exact_error}}
\end{figure}

\begin{figure}[tbph]
        \centering
        \subfigure[$\epsilon = 10^{-2}$.]{\includegraphics[width=0.3\textwidth]{figures/mc_error_verification/svd_laplace_eps_-2.eps}} 
        \subfigure[$\epsilon = 10^{-8}$.]{\includegraphics[width=0.3\textwidth]{figures/mc_error_verification/svd_laplace_eps_-8.eps}} 
        \subfigure[$\epsilon = 10^{-14}$.]{\includegraphics[width=0.3\textwidth]{figures/mc_error_verification/svd_laplace_eps_-14.eps}} 
\caption{Laplace kernel SVD compression experiments with $N = 10^6$, $m = 100$, $d = 3$, and $D_{WS} = 4$. The error is computed exactly.
\label{fig_3d_laplace_ws4_svd_exact_error}}
\end{figure}

%%%

\begin{figure}[tbph]
        \centering
        \subfigure[$\epsilon = 10^{-2}$.]{\includegraphics[width=0.3\textwidth]{figures/mc_error_verification/approx_id_gaussian_eps_-2.eps}} 
        \subfigure[$\epsilon = 10^{-8}$.]{\includegraphics[width=0.3\textwidth]{figures/mc_error_verification/approx_id_gaussian_eps_-8.eps}} 
        \subfigure[$\epsilon = 10^{-14}$.]{\includegraphics[width=0.3\textwidth]{figures/mc_error_verification/approx_id_gaussian_eps_-14.eps}} 
\caption{Gaussian kernel ID compression experiments with $N = 10^6$, $m = 100$, $d = 3$, and $D_{WS} = 4$. The error is estimated with $s = 10^{-2}$ and $n_{\textrm{MC}} =1$.
\label{fig_3d_gaussian_ws4_id_approx_error}}
\end{figure}

\begin{figure}[tbph]
        \centering
        \subfigure[$\epsilon = 10^{-2}$.]{\includegraphics[width=0.3\textwidth]{figures/mc_error_verification/approx_svd_gaussian_eps_-2.eps}} 
        \subfigure[$\epsilon = 10^{-8}$.]{\includegraphics[width=0.3\textwidth]{figures/mc_error_verification/approx_svd_gaussian_eps_-8.eps}} 
        \subfigure[$\epsilon = 10^{-14}$.]{\includegraphics[width=0.3\textwidth]{figures/mc_error_verification/approx_svd_gaussian_eps_-14.eps}} 
\caption{Gaussian kernel SVD compression experiments with $N = 10^6$, $m = 100$, $d = 3$, and $D_{WS} = 4$. The error is estimated with $s = 10^{-2}$ and $n_{\textrm{MC}} =1$.
\label{fig_3d_gaussian_ws4_svd_approx_error}}
\end{figure}

\begin{figure}[tbph]
        \centering
        \subfigure[$\epsilon = 10^{-2}$.]{\includegraphics[width=0.3\textwidth]{figures/mc_error_verification/approx_id_laplace_eps_-2.eps}} 
        \subfigure[$\epsilon = 10^{-8}$.]{\includegraphics[width=0.3\textwidth]{figures/mc_error_verification/approx_id_laplace_eps_-8.eps}} 
        \subfigure[$\epsilon = 10^{-14}$.]{\includegraphics[width=0.3\textwidth]{figures/mc_error_verification/approx_id_laplace_eps_-14.eps}} 
\caption{Laplace kernel ID compression experiments with $N = 10^6$, $m = 100$, $d = 3$, and $D_{WS} = 4$. The error is estimated with $s = 10^{-2}$ and $n_{\textrm{MC}} =1$.
\label{fig_3d_laplace_ws4_id_approx_error}}
\end{figure}

\begin{figure}[tbph]
        \centering
        \subfigure[$\epsilon = 10^{-2}$.]{\includegraphics[width=0.3\textwidth]{figures/mc_error_verification/approx_svd_laplace_eps_-2.eps}} 
        \subfigure[$\epsilon = 10^{-8}$.]{\includegraphics[width=0.3\textwidth]{figures/mc_error_verification/approx_svd_laplace_eps_-8.eps}} 
        \subfigure[$\epsilon = 10^{-14}$.]{\includegraphics[width=0.3\textwidth]{figures/mc_error_verification/approx_svd_laplace_eps_-14.eps}} 
\caption{Laplace kernel SVD compression experiments with $N = 10^6$, $m = 100$, $d = 3$, and $D_{WS} = 4$. The error is estimated with $s = 10^{-2}$ and $n_{\textrm{MC}} =1$.
\label{fig_3d_laplace_ws4_svd_approx_error}}
\end{figure}

%%%

\begin{figure}[tbph]
        \centering
        \subfigure[$\epsilon = 10^{-2}$.]{\includegraphics[width=0.3\textwidth]{figures/mc_error_verification/gaussian_smaller_ws/id_gaussian_eps_-2.eps}} 
        \subfigure[$\epsilon = 10^{-8}$.]{\includegraphics[width=0.3\textwidth]{figures/mc_error_verification/gaussian_smaller_ws/id_gaussian_eps_-8.eps}} 
        \subfigure[$\epsilon = 10^{-14}$.]{\includegraphics[width=0.3\textwidth]{figures/mc_error_verification/gaussian_smaller_ws/id_gaussian_eps_-14.eps}} 
\caption{Gaussian kernel ID compression experiments with $N = 10^6$, $m = 100$, $d = 3$, and $D_{WS} = 3$. The error is computed exactly.
\label{fig_3d_gaussian_ws3_id_exact_error}}
\end{figure}

\begin{figure}[tbph]
        \centering
        \subfigure[$\epsilon = 10^{-2}$.]{\includegraphics[width=0.3\textwidth]{figures/mc_error_verification/gaussian_smaller_ws/svd_gaussian_eps_-2.eps}} 
        \subfigure[$\epsilon = 10^{-8}$.]{\includegraphics[width=0.3\textwidth]{figures/mc_error_verification/gaussian_smaller_ws/svd_gaussian_eps_-8.eps}} 
        \subfigure[$\epsilon = 10^{-14}$.]{\includegraphics[width=0.3\textwidth]{figures/mc_error_verification/gaussian_smaller_ws/svd_gaussian_eps_-14.eps}} 
\caption{Gaussian kernel SVD compression experiments with $N = 10^6$, $m = 100$, $d = 3$, and $D_{WS} = 3$. The error is computed exactly.
\label{fig_3d_gaussian_ws3_svd_exact_error}}
\end{figure}

\begin{figure}[tbph]
        \centering
        \subfigure[$\epsilon = 10^{-2}$.]{\includegraphics[width=0.3\textwidth]{figures/mc_error_verification/gaussian_smaller_ws/approx_id_gaussian_eps_-2.eps}} 
        \subfigure[$\epsilon = 10^{-8}$.]{\includegraphics[width=0.3\textwidth]{figures/mc_error_verification/gaussian_smaller_ws/approx_id_gaussian_eps_-8.eps}} 
        \subfigure[$\epsilon = 10^{-14}$.]{\includegraphics[width=0.3\textwidth]{figures/mc_error_verification/gaussian_smaller_ws/approx_id_gaussian_eps_-14.eps}} 
\caption{Gaussian kernel ID compression experiments with $N = 10^6$, $m = 100$, $d = 3$, and $D_{WS} = 3$. The error is estimated with $s = 10^{-2}$ and $n_{\textrm{MC}} =1$.
\label{fig_3d_gaussian_ws3_id_approx_error}}
\end{figure}

\begin{figure}[tbph]
        \centering
        \subfigure[$\epsilon = 10^{-2}$.]{\includegraphics[width=0.3\textwidth]{figures/mc_error_verification/gaussian_smaller_ws/approx_svd_gaussian_eps_-2.eps}} 
        \subfigure[$\epsilon = 10^{-8}$.]{\includegraphics[width=0.3\textwidth]{figures/mc_error_verification/gaussian_smaller_ws/approx_svd_gaussian_eps_-8.eps}} 
        \subfigure[$\epsilon = 10^{-14}$.]{\includegraphics[width=0.3\textwidth]{figures/mc_error_verification/gaussian_smaller_ws/approx_svd_gaussian_eps_-14.eps}} 
\caption{Gaussian kernel SVD compression experiments with $N = 10^6$, $m = 100$, $d = 3$, and $D_{WS} = 3$. The error is estimated with $s = 10^{-2}$ and $n_{\textrm{MC}} =1$.
\label{fig_3d_gaussian_ws3_svd_approx_error}}
\end{figure}

%%%%%%%%%

\subsection{Gaussian Errors Are Not Smooth}

Note that in the new experiments, it seems that the Gaussian kernel compresses much less than the Laplace kernel. I thought this might be due to only performing the experiment once, so I did a small run with several repeats. These are the results.  

More concretely, I generate a single data set, but choose multiple centers for the set of sources and perform the experiment for each set of sources.  The results are then averaged over these experiments. The reported ranks are the rounded average over runs. 

Note that for the sampling parameter equal to $10^{-1}$, the error is always close to one. Why is this happening?

\begin{figure}[tbph]
        \centering
        \subfigure[$\epsilon = 10^{-2}$.]{\includegraphics[width=0.3\textwidth]{figures/repeats_after_mc_error/repeats_for_smoothness/id_gaussian_eps_-2.eps}} 
        \subfigure[$\epsilon = 10^{-8}$.]{\includegraphics[width=0.3\textwidth]{figures/repeats_after_mc_error/repeats_for_smoothness/id_gaussian_eps_-8.eps}} 
        \subfigure[$\epsilon = 10^{-14}$.]{\includegraphics[width=0.3\textwidth]{figures/repeats_after_mc_error/repeats_for_smoothness/id_gaussian_eps_-14.eps}} 
\caption{Gaussian kernel ID compression experiments with $N = 10^6$, $m = 100$, $d = 3$, and $D_{WS} = 3$. The error is computed exactly, and the errors are averaged over 10 repeats of the experiment. 
\label{fig_3d_gaussian_ws3_id_smoothness_repeats}}
\end{figure}

%%%%%%%%%%%%%%%%%%%%%%%%%%%%%%%%%%%%%%%%%%%%%%%%%%%%%%%%%%%%%%%%%%
%%%%%%%%%%%%%%%%%%%%%%%%%%%%%%%%%%%%%%%%%%%%%%%%%%%%%%%%%%%%%%%%%%
%%%%%%%%%%%%%%%%%%%%%%%%%%%%%%%%%%%%%%%%%%%%%%%%%%%%%%%%%%%%%%%%%%

\subsection{Larger Numbers of Sources}

Equipped with the MC error estimator described above, we can now perform compression experiments on larger numbers of sources.  The goal here is to determine if we really aren't getting any compression or if the true rank is just larger than 100.  

\begin{figure}[tbph]
        \centering
        \subfigure[$m = 100$.]{\includegraphics[width=0.3\textwidth]{figures/large_leaves/approx_id_gaussian_eps_-2_leaf_100.eps}} 
        \subfigure[$m = 200$.]{\includegraphics[width=0.3\textwidth]{figures/large_leaves/approx_id_gaussian_eps_-2_leaf_200.eps}} 
        \subfigure[$m = 300$.]{\includegraphics[width=0.3\textwidth]{figures/large_leaves/approx_id_gaussian_eps_-2_leaf_300.eps}} 
        \subfigure[$m = 400$.]{\includegraphics[width=0.3\textwidth]{figures/large_leaves/approx_id_gaussian_eps_-2_leaf_400.eps}} 
        \subfigure[$m = 500$.]{\includegraphics[width=0.3\textwidth]{figures/large_leaves/approx_id_gaussian_eps_-2_leaf_500.eps}} 
        \subfigure[$m = 600$.]{\includegraphics[width=0.3\textwidth]{figures/large_leaves/approx_id_gaussian_eps_-2_leaf_600.eps}} 
        \subfigure[$m = 700$.]{\includegraphics[width=0.3\textwidth]{figures/large_leaves/approx_id_gaussian_eps_-2_leaf_700.eps}} 
        \subfigure[$m = 800$.]{\includegraphics[width=0.3\textwidth]{figures/large_leaves/approx_id_gaussian_eps_-2_leaf_800.eps}} 
        \subfigure[$m = 900$.]{\includegraphics[width=0.3\textwidth]{figures/large_leaves/approx_id_gaussian_eps_-2_leaf_900.eps}} 
        \subfigure[$m = 1000$.]{\includegraphics[width=0.3\textwidth]{figures/large_leaves/approx_id_gaussian_eps_-2_leaf_1000.eps}} 
\caption{Gaussian kernel ID compression experiments with $N = 10^6$, $\epsilon = 10^{-2}$, $d = 3$, and $D_{WS} = 4$. The error is computed approximately with $s = 10^{-2}$ and $n_{\textrm{MC}} = 5$. 
\label{fig_large_leaves_3d_gaussian_ws4_id_eps2}}
\end{figure}

\begin{figure}[tbph]
        \centering
        \subfigure[$m = 100$.]{\includegraphics[width=0.3\textwidth]{figures/large_leaves/approx_id_gaussian_eps_-8_leaf_100.eps}} 
        \subfigure[$m = 200$.]{\includegraphics[width=0.3\textwidth]{figures/large_leaves/approx_id_gaussian_eps_-8_leaf_200.eps}} 
        \subfigure[$m = 300$.]{\includegraphics[width=0.3\textwidth]{figures/large_leaves/approx_id_gaussian_eps_-8_leaf_300.eps}} 
        \subfigure[$m = 400$.]{\includegraphics[width=0.3\textwidth]{figures/large_leaves/approx_id_gaussian_eps_-8_leaf_400.eps}} 
        \subfigure[$m = 500$.]{\includegraphics[width=0.3\textwidth]{figures/large_leaves/approx_id_gaussian_eps_-8_leaf_500.eps}} 
        \subfigure[$m = 600$.]{\includegraphics[width=0.3\textwidth]{figures/large_leaves/approx_id_gaussian_eps_-8_leaf_600.eps}} 
        \subfigure[$m = 700$.]{\includegraphics[width=0.3\textwidth]{figures/large_leaves/approx_id_gaussian_eps_-8_leaf_700.eps}} 
        \subfigure[$m = 800$.]{\includegraphics[width=0.3\textwidth]{figures/large_leaves/approx_id_gaussian_eps_-8_leaf_800.eps}} 
        \subfigure[$m = 900$.]{\includegraphics[width=0.3\textwidth]{figures/large_leaves/approx_id_gaussian_eps_-8_leaf_900.eps}} 
        \subfigure[$m = 1000$.]{\includegraphics[width=0.3\textwidth]{figures/large_leaves/approx_id_gaussian_eps_-8_leaf_1000.eps}} 
\caption{Gaussian kernel ID compression experiments with $N = 10^6$, $\epsilon = 10^{-8}$, $d = 3$, and $D_{WS} = 4$. The error is computed approximately with $s = 10^{-2}$ and $n_{\textrm{MC}} = 5$. 
\label{fig_large_leaves_3d_gaussian_ws4_id_eps8}}
\end{figure}

\begin{figure}[tbph]
        \centering
        \subfigure[$m = 100$.]{\includegraphics[width=0.3\textwidth]{figures/large_leaves/approx_id_gaussian_eps_-14_leaf_100.eps}} 
        \subfigure[$m = 200$.]{\includegraphics[width=0.3\textwidth]{figures/large_leaves/approx_id_gaussian_eps_-14_leaf_200.eps}} 
        \subfigure[$m = 300$.]{\includegraphics[width=0.3\textwidth]{figures/large_leaves/approx_id_gaussian_eps_-14_leaf_300.eps}} 
        \subfigure[$m = 400$.]{\includegraphics[width=0.3\textwidth]{figures/large_leaves/approx_id_gaussian_eps_-14_leaf_400.eps}} 
        \subfigure[$m = 500$.]{\includegraphics[width=0.3\textwidth]{figures/large_leaves/approx_id_gaussian_eps_-14_leaf_500.eps}} 
        \subfigure[$m = 600$.]{\includegraphics[width=0.3\textwidth]{figures/large_leaves/approx_id_gaussian_eps_-14_leaf_600.eps}} 
        \subfigure[$m = 700$.]{\includegraphics[width=0.3\textwidth]{figures/large_leaves/approx_id_gaussian_eps_-14_leaf_700.eps}} 
        \subfigure[$m = 800$.]{\includegraphics[width=0.3\textwidth]{figures/large_leaves/approx_id_gaussian_eps_-14_leaf_800.eps}} 
        \subfigure[$m = 900$.]{\includegraphics[width=0.3\textwidth]{figures/large_leaves/approx_id_gaussian_eps_-14_leaf_900.eps}} 
        \subfigure[$m = 1000$.]{\includegraphics[width=0.3\textwidth]{figures/large_leaves/approx_id_gaussian_eps_-14_leaf_1000.eps}} 
\caption{Gaussian kernel ID compression experiments with $N = 10^6$, $\epsilon = 10^{-14}$, $d = 3$, and $D_{WS} = 4$. The error is computed approximately with $s = 10^{-2}$ and $n_{\textrm{MC}} = 5$. 
\label{fig_large_leaves_3d_gaussian_ws4_id_eps14}}
\end{figure}

\begin{figure}[tbph]
        \centering
        \subfigure[$m = 100$.]{\includegraphics[width=0.3\textwidth]{figures/large_leaves/approx_svd_gaussian_eps_-2_leaf_100.eps}} 
        \subfigure[$m = 200$.]{\includegraphics[width=0.3\textwidth]{figures/large_leaves/approx_svd_gaussian_eps_-2_leaf_200.eps}} 
        \subfigure[$m = 300$.]{\includegraphics[width=0.3\textwidth]{figures/large_leaves/approx_svd_gaussian_eps_-2_leaf_300.eps}} 
        \subfigure[$m = 400$.]{\includegraphics[width=0.3\textwidth]{figures/large_leaves/approx_svd_gaussian_eps_-2_leaf_400.eps}} 
        \subfigure[$m = 500$.]{\includegraphics[width=0.3\textwidth]{figures/large_leaves/approx_svd_gaussian_eps_-2_leaf_500.eps}} 
        \subfigure[$m = 600$.]{\includegraphics[width=0.3\textwidth]{figures/large_leaves/approx_svd_gaussian_eps_-2_leaf_600.eps}} 
        \subfigure[$m = 700$.]{\includegraphics[width=0.3\textwidth]{figures/large_leaves/approx_svd_gaussian_eps_-2_leaf_700.eps}} 
        \subfigure[$m = 800$.]{\includegraphics[width=0.3\textwidth]{figures/large_leaves/approx_svd_gaussian_eps_-2_leaf_800.eps}} 
        \subfigure[$m = 900$.]{\includegraphics[width=0.3\textwidth]{figures/large_leaves/approx_svd_gaussian_eps_-2_leaf_900.eps}} 
        \subfigure[$m = 1000$.]{\includegraphics[width=0.3\textwidth]{figures/large_leaves/approx_svd_gaussian_eps_-2_leaf_1000.eps}} 
\caption{Gaussian kernel SVD compression experiments with $N = 10^6$, $\epsilon = 10^{-2}$, $d = 3$, and $D_{WS} = 4$. The error is computed approximately with $s = 10^{-2}$ and $n_{\textrm{MC}} = 5$. 
\label{fig_large_leaves_3d_gaussian_ws4_svd_eps2}}
\end{figure}

\begin{figure}[tbph]
        \centering
        \subfigure[$m = 100$.]{\includegraphics[width=0.3\textwidth]{figures/large_leaves/approx_svd_gaussian_eps_-8_leaf_100.eps}} 
        \subfigure[$m = 200$.]{\includegraphics[width=0.3\textwidth]{figures/large_leaves/approx_svd_gaussian_eps_-8_leaf_200.eps}} 
        \subfigure[$m = 300$.]{\includegraphics[width=0.3\textwidth]{figures/large_leaves/approx_svd_gaussian_eps_-8_leaf_300.eps}} 
        \subfigure[$m = 400$.]{\includegraphics[width=0.3\textwidth]{figures/large_leaves/approx_svd_gaussian_eps_-8_leaf_400.eps}} 
        \subfigure[$m = 500$.]{\includegraphics[width=0.3\textwidth]{figures/large_leaves/approx_svd_gaussian_eps_-8_leaf_500.eps}} 
        \subfigure[$m = 600$.]{\includegraphics[width=0.3\textwidth]{figures/large_leaves/approx_svd_gaussian_eps_-8_leaf_600.eps}} 
        \subfigure[$m = 700$.]{\includegraphics[width=0.3\textwidth]{figures/large_leaves/approx_svd_gaussian_eps_-8_leaf_700.eps}} 
        \subfigure[$m = 800$.]{\includegraphics[width=0.3\textwidth]{figures/large_leaves/approx_svd_gaussian_eps_-8_leaf_800.eps}} 
        \subfigure[$m = 900$.]{\includegraphics[width=0.3\textwidth]{figures/large_leaves/approx_svd_gaussian_eps_-8_leaf_900.eps}} 
        \subfigure[$m = 1000$.]{\includegraphics[width=0.3\textwidth]{figures/large_leaves/approx_svd_gaussian_eps_-8_leaf_1000.eps}} 
\caption{Gaussian kernel SVD compression experiments with $N = 10^6$, $\epsilon = 10^{-8}$, $d = 3$, and $D_{WS} = 4$. The error is computed approximately with $s = 10^{-2}$ and $n_{\textrm{MC}} = 5$. 
\label{fig_large_leaves_3d_gaussian_ws4_svd_eps8}}
\end{figure}

\begin{figure}[tbph]
        \centering
        \subfigure[$m = 100$.]{\includegraphics[width=0.3\textwidth]{figures/large_leaves/approx_svd_gaussian_eps_-14_leaf_100.eps}} 
        \subfigure[$m = 200$.]{\includegraphics[width=0.3\textwidth]{figures/large_leaves/approx_svd_gaussian_eps_-14_leaf_200.eps}} 
        \subfigure[$m = 300$.]{\includegraphics[width=0.3\textwidth]{figures/large_leaves/approx_svd_gaussian_eps_-14_leaf_300.eps}} 
        \subfigure[$m = 400$.]{\includegraphics[width=0.3\textwidth]{figures/large_leaves/approx_svd_gaussian_eps_-14_leaf_400.eps}} 
        \subfigure[$m = 500$.]{\includegraphics[width=0.3\textwidth]{figures/large_leaves/approx_svd_gaussian_eps_-14_leaf_500.eps}} 
        \subfigure[$m = 600$.]{\includegraphics[width=0.3\textwidth]{figures/large_leaves/approx_svd_gaussian_eps_-14_leaf_600.eps}} 
        \subfigure[$m = 700$.]{\includegraphics[width=0.3\textwidth]{figures/large_leaves/approx_svd_gaussian_eps_-14_leaf_700.eps}} 
        \subfigure[$m = 800$.]{\includegraphics[width=0.3\textwidth]{figures/large_leaves/approx_svd_gaussian_eps_-14_leaf_800.eps}} 
        \subfigure[$m = 900$.]{\includegraphics[width=0.3\textwidth]{figures/large_leaves/approx_svd_gaussian_eps_-14_leaf_900.eps}} 
        \subfigure[$m = 1000$.]{\includegraphics[width=0.3\textwidth]{figures/large_leaves/approx_svd_gaussian_eps_-14_leaf_1000.eps}} 
\caption{Gaussian kernel SVD compression experiments with $N = 10^6$, $\epsilon = 10^{-14}$, $d = 3$, and $D_{WS} = 4$. The error is computed approximately with $s = 10^{-2}$ and $n_{\textrm{MC}} = 5$. 
\label{fig_large_leaves_3d_gaussian_ws4_svd_eps14}}
\end{figure}

%%%%%

\begin{figure}[tbph]
        \centering
        \subfigure[$m = 100$.]{\includegraphics[width=0.3\textwidth]{figures/large_leaves/approx_id_laplace_eps_-2_leaf_100.eps}} 
        \subfigure[$m = 200$.]{\includegraphics[width=0.3\textwidth]{figures/large_leaves/approx_id_laplace_eps_-2_leaf_200.eps}} 
        \subfigure[$m = 300$.]{\includegraphics[width=0.3\textwidth]{figures/large_leaves/approx_id_laplace_eps_-2_leaf_300.eps}} 
        \subfigure[$m = 400$.]{\includegraphics[width=0.3\textwidth]{figures/large_leaves/approx_id_laplace_eps_-2_leaf_400.eps}} 
        \subfigure[$m = 500$.]{\includegraphics[width=0.3\textwidth]{figures/large_leaves/approx_id_laplace_eps_-2_leaf_500.eps}} 
        \subfigure[$m = 600$.]{\includegraphics[width=0.3\textwidth]{figures/large_leaves/approx_id_laplace_eps_-2_leaf_600.eps}} 
        \subfigure[$m = 700$.]{\includegraphics[width=0.3\textwidth]{figures/large_leaves/approx_id_laplace_eps_-2_leaf_700.eps}} 
        \subfigure[$m = 800$.]{\includegraphics[width=0.3\textwidth]{figures/large_leaves/approx_id_laplace_eps_-2_leaf_800.eps}} 
        \subfigure[$m = 900$.]{\includegraphics[width=0.3\textwidth]{figures/large_leaves/approx_id_laplace_eps_-2_leaf_900.eps}} 
        \subfigure[$m = 1000$.]{\includegraphics[width=0.3\textwidth]{figures/large_leaves/approx_id_laplace_eps_-2_leaf_1000.eps}} 
\caption{Laplace kernel ID compression experiments with $N = 10^6$, $\epsilon = 10^{-2}$, $d = 3$, and $D_{WS} = 4$. The error is computed approximately with $s = 10^{-2}$ and $n_{\textrm{MC}} = 5$. 
\label{fig_large_leaves_3d_laplace_ws4_id_eps2}}
\end{figure}

\begin{figure}[tbph]
        \centering
        \subfigure[$m = 100$.]{\includegraphics[width=0.3\textwidth]{figures/large_leaves/approx_id_laplace_eps_-8_leaf_100.eps}} 
        \subfigure[$m = 200$.]{\includegraphics[width=0.3\textwidth]{figures/large_leaves/approx_id_laplace_eps_-8_leaf_200.eps}} 
        \subfigure[$m = 300$.]{\includegraphics[width=0.3\textwidth]{figures/large_leaves/approx_id_laplace_eps_-8_leaf_300.eps}} 
        \subfigure[$m = 400$.]{\includegraphics[width=0.3\textwidth]{figures/large_leaves/approx_id_laplace_eps_-8_leaf_400.eps}} 
        \subfigure[$m = 500$.]{\includegraphics[width=0.3\textwidth]{figures/large_leaves/approx_id_laplace_eps_-8_leaf_500.eps}} 
        \subfigure[$m = 600$.]{\includegraphics[width=0.3\textwidth]{figures/large_leaves/approx_id_laplace_eps_-8_leaf_600.eps}} 
        \subfigure[$m = 700$.]{\includegraphics[width=0.3\textwidth]{figures/large_leaves/approx_id_laplace_eps_-8_leaf_700.eps}} 
        \subfigure[$m = 800$.]{\includegraphics[width=0.3\textwidth]{figures/large_leaves/approx_id_laplace_eps_-8_leaf_800.eps}} 
        \subfigure[$m = 900$.]{\includegraphics[width=0.3\textwidth]{figures/large_leaves/approx_id_laplace_eps_-8_leaf_900.eps}} 
        \subfigure[$m = 1000$.]{\includegraphics[width=0.3\textwidth]{figures/large_leaves/approx_id_laplace_eps_-8_leaf_1000.eps}} 
\caption{Laplace kernel ID compression experiments with $N = 10^6$, $\epsilon = 10^{-8}$, $d = 3$, and $D_{WS} = 4$. The error is computed approximately with $s = 10^{-2}$ and $n_{\textrm{MC}} = 5$. 
\label{fig_large_leaves_3d_laplace_ws4_id_eps8}}
\end{figure}

\begin{figure}[tbph]
        \centering
        \subfigure[$m = 100$.]{\includegraphics[width=0.3\textwidth]{figures/large_leaves/approx_id_laplace_eps_-14_leaf_100.eps}} 
        \subfigure[$m = 200$.]{\includegraphics[width=0.3\textwidth]{figures/large_leaves/approx_id_laplace_eps_-14_leaf_200.eps}} 
        \subfigure[$m = 300$.]{\includegraphics[width=0.3\textwidth]{figures/large_leaves/approx_id_laplace_eps_-14_leaf_300.eps}} 
        \subfigure[$m = 400$.]{\includegraphics[width=0.3\textwidth]{figures/large_leaves/approx_id_laplace_eps_-14_leaf_400.eps}} 
        \subfigure[$m = 500$.]{\includegraphics[width=0.3\textwidth]{figures/large_leaves/approx_id_laplace_eps_-14_leaf_500.eps}} 
        \subfigure[$m = 600$.]{\includegraphics[width=0.3\textwidth]{figures/large_leaves/approx_id_laplace_eps_-14_leaf_600.eps}} 
        \subfigure[$m = 700$.]{\includegraphics[width=0.3\textwidth]{figures/large_leaves/approx_id_laplace_eps_-14_leaf_700.eps}} 
        \subfigure[$m = 800$.]{\includegraphics[width=0.3\textwidth]{figures/large_leaves/approx_id_laplace_eps_-14_leaf_800.eps}} 
        \subfigure[$m = 900$.]{\includegraphics[width=0.3\textwidth]{figures/large_leaves/approx_id_laplace_eps_-14_leaf_900.eps}} 
        \subfigure[$m = 1000$.]{\includegraphics[width=0.3\textwidth]{figures/large_leaves/approx_id_laplace_eps_-14_leaf_1000.eps}} 
\caption{Laplace kernel ID compression experiments with $N = 10^6$, $\epsilon = 10^{-14}$, $d = 3$, and $D_{WS} = 4$. The error is computed approximately with $s = 10^{-2}$ and $n_{\textrm{MC}} = 5$. 
\label{fig_large_leaves_3d_laplace_ws4_id_eps14}}
\end{figure}

%%%

\begin{figure}[tbph]
        \centering
        \subfigure[$m = 100$.]{\includegraphics[width=0.3\textwidth]{figures/large_leaves/approx_svd_laplace_eps_-2_leaf_100.eps}} 
        \subfigure[$m = 200$.]{\includegraphics[width=0.3\textwidth]{figures/large_leaves/approx_svd_laplace_eps_-2_leaf_200.eps}} 
        \subfigure[$m = 300$.]{\includegraphics[width=0.3\textwidth]{figures/large_leaves/approx_svd_laplace_eps_-2_leaf_300.eps}} 
        \subfigure[$m = 400$.]{\includegraphics[width=0.3\textwidth]{figures/large_leaves/approx_svd_laplace_eps_-2_leaf_400.eps}} 
        \subfigure[$m = 500$.]{\includegraphics[width=0.3\textwidth]{figures/large_leaves/approx_svd_laplace_eps_-2_leaf_500.eps}} 
        \subfigure[$m = 600$.]{\includegraphics[width=0.3\textwidth]{figures/large_leaves/approx_svd_laplace_eps_-2_leaf_600.eps}} 
        \subfigure[$m = 700$.]{\includegraphics[width=0.3\textwidth]{figures/large_leaves/approx_svd_laplace_eps_-2_leaf_700.eps}} 
        \subfigure[$m = 800$.]{\includegraphics[width=0.3\textwidth]{figures/large_leaves/approx_svd_laplace_eps_-2_leaf_800.eps}} 
        \subfigure[$m = 900$.]{\includegraphics[width=0.3\textwidth]{figures/large_leaves/approx_svd_laplace_eps_-2_leaf_900.eps}} 
        \subfigure[$m = 1000$.]{\includegraphics[width=0.3\textwidth]{figures/large_leaves/approx_svd_laplace_eps_-2_leaf_1000.eps}} 
\caption{Laplace kernel SVD compression experiments with $N = 10^6$, $\epsilon = 10^{-2}$, $d = 3$, and $D_{WS} = 4$. The error is computed approximately with $s = 10^{-2}$ and $n_{\textrm{MC}} = 5$. 
\label{fig_large_leaves_3d_laplace_ws4_svd_eps2}}
\end{figure}

\begin{figure}[tbph]
        \centering
        \subfigure[$m = 100$.]{\includegraphics[width=0.3\textwidth]{figures/large_leaves/approx_svd_laplace_eps_-8_leaf_100.eps}} 
        \subfigure[$m = 200$.]{\includegraphics[width=0.3\textwidth]{figures/large_leaves/approx_svd_laplace_eps_-8_leaf_200.eps}} 
        \subfigure[$m = 300$.]{\includegraphics[width=0.3\textwidth]{figures/large_leaves/approx_svd_laplace_eps_-8_leaf_300.eps}} 
        \subfigure[$m = 400$.]{\includegraphics[width=0.3\textwidth]{figures/large_leaves/approx_svd_laplace_eps_-8_leaf_400.eps}} 
        \subfigure[$m = 500$.]{\includegraphics[width=0.3\textwidth]{figures/large_leaves/approx_svd_laplace_eps_-8_leaf_500.eps}} 
        \subfigure[$m = 600$.]{\includegraphics[width=0.3\textwidth]{figures/large_leaves/approx_svd_laplace_eps_-8_leaf_600.eps}} 
        \subfigure[$m = 700$.]{\includegraphics[width=0.3\textwidth]{figures/large_leaves/approx_svd_laplace_eps_-8_leaf_700.eps}} 
        \subfigure[$m = 800$.]{\includegraphics[width=0.3\textwidth]{figures/large_leaves/approx_svd_laplace_eps_-8_leaf_800.eps}} 
        \subfigure[$m = 900$.]{\includegraphics[width=0.3\textwidth]{figures/large_leaves/approx_svd_laplace_eps_-8_leaf_900.eps}} 
        \subfigure[$m = 1000$.]{\includegraphics[width=0.3\textwidth]{figures/large_leaves/approx_svd_laplace_eps_-8_leaf_1000.eps}} 
\caption{Laplace kernel SVD compression experiments with $N = 10^6$, $\epsilon = 10^{-8}$, $d = 3$, and $D_{WS} = 4$. The error is computed approximately with $s = 10^{-2}$ and $n_{\textrm{MC}} = 5$. 
\label{fig_large_leaves_3d_laplace_ws4_svd_eps8}}
\end{figure}

\begin{figure}[tbph]
        \centering
        \subfigure[$m = 100$.]{\includegraphics[width=0.3\textwidth]{figures/large_leaves/approx_svd_laplace_eps_-14_leaf_100.eps}} 
        \subfigure[$m = 200$.]{\includegraphics[width=0.3\textwidth]{figures/large_leaves/approx_svd_laplace_eps_-14_leaf_200.eps}} 
        \subfigure[$m = 300$.]{\includegraphics[width=0.3\textwidth]{figures/large_leaves/approx_svd_laplace_eps_-14_leaf_300.eps}} 
        \subfigure[$m = 400$.]{\includegraphics[width=0.3\textwidth]{figures/large_leaves/approx_svd_laplace_eps_-14_leaf_400.eps}} 
        \subfigure[$m = 500$.]{\includegraphics[width=0.3\textwidth]{figures/large_leaves/approx_svd_laplace_eps_-14_leaf_500.eps}} 
        \subfigure[$m = 600$.]{\includegraphics[width=0.3\textwidth]{figures/large_leaves/approx_svd_laplace_eps_-14_leaf_600.eps}} 
        \subfigure[$m = 700$.]{\includegraphics[width=0.3\textwidth]{figures/large_leaves/approx_svd_laplace_eps_-14_leaf_700.eps}} 
        \subfigure[$m = 800$.]{\includegraphics[width=0.3\textwidth]{figures/large_leaves/approx_svd_laplace_eps_-14_leaf_800.eps}} 
        \subfigure[$m = 900$.]{\includegraphics[width=0.3\textwidth]{figures/large_leaves/approx_svd_laplace_eps_-14_leaf_900.eps}} 
        \subfigure[$m = 1000$.]{\includegraphics[width=0.3\textwidth]{figures/large_leaves/approx_svd_laplace_eps_-14_leaf_1000.eps}} 
\caption{Laplace kernel SVD compression experiments with $N = 10^6$, $\epsilon = 10^{-14}$, $d = 3$, and $D_{WS} = 4$. The error is computed approximately with $s = 10^{-2}$ and $n_{\textrm{MC}} = 5$. 
\label{fig_large_leaves_3d_laplace_ws4_svd_eps14}}
\end{figure}

%%%%%%%%%%%%%%%%%%%%%%%%%%%%%%%%%%%%%%%%%%%%%%%%%%%%%%%%%%%%%%%%

%% Laplace kernel

\begin{figure}[tbph]
        \centering
        \subfigure[$\epsilon = 10^{-2}$.]{\includegraphics[width=0.3\textwidth]{figures/repeats_after_mc_error/id_laplace_eps_-2_d_1.eps}} 
        \subfigure[$\epsilon = 10^{-8}$.]{\includegraphics[width=0.3\textwidth]{figures/repeats_after_mc_error/id_laplace_eps_-8_d_1.eps}} 
        \subfigure[$\epsilon = 10^{-14}$.]{\includegraphics[width=0.3\textwidth]{figures/repeats_after_mc_error/id_laplace_eps_-14_d_1.eps}} 
\caption{Laplace kernel compression experiments with $N = 10^6$, $m = 100$, $d = 1$, and $D_{WS} = 3$. 
\label{fig_1d_laplace_ws3_redo}}
\end{figure}

\begin{figure}[tbph]
        \centering
        \subfigure[$\epsilon = 10^{-2}$.]{\includegraphics[width=0.3\textwidth]{figures/repeats_after_mc_error/id_laplace_eps_-2_d_2.eps}} 
        \subfigure[$\epsilon = 10^{-8}$.]{\includegraphics[width=0.3\textwidth]{figures/repeats_after_mc_error/id_laplace_eps_-8_d_2.eps}} 
        \subfigure[$\epsilon = 10^{-14}$.]{\includegraphics[width=0.3\textwidth]{figures/repeats_after_mc_error/id_laplace_eps_-14_d_2.eps}} 
\caption{Laplace kernel compression experiments with $N = 10^6$, $m = 100$, $d = 2$, and $D_{WS} = 3$. 
\label{fig_2d_laplace_ws3_redo}}
\end{figure}

\begin{figure}[tbph]
        \centering
        \subfigure[$\epsilon = 10^{-2}$.]{\includegraphics[width=0.3\textwidth]{figures/repeats_after_mc_error/id_laplace_eps_-2_d_3.eps}} 
        \subfigure[$\epsilon = 10^{-8}$.]{\includegraphics[width=0.3\textwidth]{figures/repeats_after_mc_error/id_laplace_eps_-8_d_3.eps}} 
        \subfigure[$\epsilon = 10^{-14}$.]{\includegraphics[width=0.3\textwidth]{figures/repeats_after_mc_error/id_laplace_eps_-14_d_3.eps}} 
\caption{Laplace kernel compression experiments with $N = 10^6$, $m = 100$, $d = 3$, and $D_{WS} = 3$. 
\label{fig_3d_laplace_ws3_redo}}
\end{figure}

\begin{figure}[tbph]
        \centering
        \subfigure[$\epsilon = 10^{-2}$.]{\includegraphics[width=0.3\textwidth]{figures/repeats_after_mc_error/id_laplace_eps_-2_d_4.eps}} 
        \subfigure[$\epsilon = 10^{-8}$.]{\includegraphics[width=0.3\textwidth]{figures/repeats_after_mc_error/id_laplace_eps_-8_d_4.eps}} 
        \subfigure[$\epsilon = 10^{-14}$.]{\includegraphics[width=0.3\textwidth]{figures/repeats_after_mc_error/id_laplace_eps_-14_d_4.eps}} 
\caption{Laplace kernel compression experiments with $N = 10^6$, $m = 100$, $d = 4$, and $D_{WS} = 3$. 
\label{fig_4d_laplace_ws3_redo}}
\end{figure}

\begin{figure}[tbph]
        \centering
        \subfigure[$\epsilon = 10^{-2}$.]{\includegraphics[width=0.3\textwidth]{figures/repeats_after_mc_error/id_laplace_eps_-2_d_5.eps}} 
        \subfigure[$\epsilon = 10^{-8}$.]{\includegraphics[width=0.3\textwidth]{figures/repeats_after_mc_error/id_laplace_eps_-8_d_5.eps}} 
        \subfigure[$\epsilon = 10^{-14}$.]{\includegraphics[width=0.3\textwidth]{figures/repeats_after_mc_error/id_laplace_eps_-14_d_5.eps}} 
\caption{Laplace kernel compression experiments with $N = 10^6$, $m = 100$, $d = 5$, and $D_{WS} = 3$. 
\label{fig_5d_laplace_ws3_redo}}
\end{figure}

\begin{figure}[tbph]
        \centering
        \subfigure[$\epsilon = 10^{-2}$.]{\includegraphics[width=0.3\textwidth]{figures/repeats_after_mc_error/id_laplace_eps_-2_d_8.eps}} 
        \subfigure[$\epsilon = 10^{-8}$.]{\includegraphics[width=0.3\textwidth]{figures/repeats_after_mc_error/id_laplace_eps_-8_d_8.eps}} 
        \subfigure[$\epsilon = 10^{-14}$.]{\includegraphics[width=0.3\textwidth]{figures/repeats_after_mc_error/id_laplace_eps_-14_d_8.eps}} 
\caption{Laplace kernel compression experiments with $N = 10^6$, $m = 100$, $d = 8$, and $D_{WS} = 3$. 
\label{fig_8d_laplace_ws3_redo}}
\end{figure}

\begin{figure}[tbph]
        \centering
        \subfigure[$\epsilon = 10^{-2}$.]{\includegraphics[width=0.3\textwidth]{figures/repeats_after_mc_error/id_laplace_eps_-2_d_10.eps}} 
        \subfigure[$\epsilon = 10^{-8}$.]{\includegraphics[width=0.3\textwidth]{figures/repeats_after_mc_error/id_laplace_eps_-8_d_10.eps}} 
        \subfigure[$\epsilon = 10^{-14}$.]{\includegraphics[width=0.3\textwidth]{figures/repeats_after_mc_error/id_laplace_eps_-14_d_10.eps}} 
\caption{Laplace kernel compression experiments with $N = 10^6$, $m = 100$, $d = 10$, and $D_{WS} = 3$. 
\label{fig_10d_laplace_ws3_redo}}
\end{figure}

\begin{figure}[tbph]
        \centering
        \subfigure[$\epsilon = 10^{-2}$.]{\includegraphics[width=0.3\textwidth]{figures/repeats_after_mc_error/id_laplace_eps_-2_d_15.eps}} 
        \subfigure[$\epsilon = 10^{-8}$.]{\includegraphics[width=0.3\textwidth]{figures/repeats_after_mc_error/id_laplace_eps_-8_d_15.eps}} 
        \subfigure[$\epsilon = 10^{-14}$.]{\includegraphics[width=0.3\textwidth]{figures/repeats_after_mc_error/id_laplace_eps_-14_d_15.eps}} 
\caption{Laplace kernel compression experiments with $N = 10^6$, $m = 100$, $d = 15$, and $D_{WS} = 3$. 
\label{fig_15d_laplace_ws3_redo}}
\end{figure}

%%%%%%%%%%%%%%%%%%%%%%%

\subsection{Weird Hump in the Euclidean and Leverage Sampling Experiments}

For sampling parameters of $10^{-2}$ and $10^{-1}$, the error tends to go up while the rank of the approximation also increases.  I think this is a bug, but George isn't sure.  

These experiments use the same data set for each sampling method, and choose the origin as the starting point for the set of sources. Therefore, for each data point, the targets and sources are identical. The only thing that changes is the sampling method used and the parameters.

\begin{figure}[htbp]
\centering
\includegraphics[width=0.9\textwidth]{figures/less_randomness/approx_id_gaussian_eps_-2_N_100000_leaf_500.eps}
\caption{Gaussian kernel ID  with $N = 10^5, m = 500, d = 3, D_{WS} = 4$.  The targets and sources used for each experiment are identical.
\label{fig_3d_fixed_center_id_gaussian}}
\end{figure}

\begin{figure}[htbp]
\centering
\includegraphics[width=0.9\textwidth]{figures/less_randomness/approx_svd_gaussian_eps_-2_N_100000_leaf_500.eps}
\caption{Gaussian kernel SVD  with $N = 10^5, m = 500, d = 3, D_{WS} = 4$.  The targets and sources used for each experiment are identical.
\label{fig_3d_fixed_center_svd_gaussian}}
\end{figure}

%%%%%%%%%%%%%%%%%%%%%%%%%%%%%%%%%%%%%%%%%%%%%%%%%%%%%%%%%%%%%%%%%%
%%%%%%%%%%%%%%%%%%%%%%%%%%%%%%%%%%%%%%%%%%%%%%%%%%%%%%%%%%%%%%%%%%
%%%%%%%%%%%%%%%%%%%%%%%%%%%%%%%%%%%%%%%%%%%%%%%%%%%%%%%%%%%%%%%%%%

\subsection{Future Experiments}

Possible kernels to look at:
\begin{itemize}
\item Epanechnikov -- has asymptotic bandwidth in Silverman too, start here
\item Triangular kernel
\item Thin plate kernel
\item Fisher kernel 
\item Graph and string kernels
\item molecule kernels
\item polynomial kernels
\end{itemize}

Experiments with dimensionality:
\begin{itemize}
\item Use some real application data
\item Artificially generate low intrinsic dimensional data -- i.e. $d$ dimensional Gaussian, rotated into $D$ dimensions, plus some small  noise term. 
\end{itemize}
